# Supplementary material for: Doubly Robust Proximal Causal Learning for Continuous Treatments
Source: arXiv:2309.12819 source file (2024-03-11)
Supplement: Supplementary file 1 [file appendixD.tex]

\section{Counterexample}
Often, one may  wish for Assumption~\ref{assum:bridge} hold simultaneously, rather than separately. Then, all two identification formulas and corresponding estimators can then be applied, or considered semiparametrically efficient estimation. Unfortunately, however, it does happen that Assumption~\ref{assum:bridge}(1) does not hold, but Assumption~\ref{assum:bridge}(2) holds. Therefore, it is  necessary to generalize the proximal-IPW($q$) to the continuous case, as well as the proximal-DR generalization to the continuous case.

Note that completeness makes solving the following equation~\ref{eq.uh} and~\ref{eq.uq} become solving Eq.~\ref{eq.h} and~\ref{eq.q}:
\begin{equation}\label{eq.uh}
\mathbb{E}[Y-h(U,A,X)|A,U,X]=0
\end{equation}
\begin{equation}\label{eq.uq}
    \mathbb{E}\left[q(Z,a,X)-\dfrac{1}{f(A=a|U,X)}|U,A=a,X\right]
\end{equation}

Let us consider a simplified setting where $Y\in \{0,1\},A\in\{0,1\}$ and the variables $W, Z, U$ are all discrete variables. For any $a$, let $\mathcal{P}\left(\mathbf{W}\mid \mathbf{U},a\right)$ denote a $|\mathcal{W}|\times|\mathcal{U}|$ matrix whose $(i, s)$th element is $\mathbb{P}\left[W=w_i\mid U=u_s,A=a\right]$, $\mathcal{P}(\mathbf{Z}\mid\mathbf{U},a)$ a $|\mathcal{Z}|\times|\mathcal{U}|$ matrix whose $(j, s)$th element is $\mathbb{P}\left[Z=z_j\mid U=u_s,A=a\right]$, $\mathbb{E}\left[Y\mid\mathbf{U},a\right]$ a $1\times|\mathcal{U}|$ vector whose sth element is $\mathbb{E}\left[Y\mid U=u_{s},A=a\right]$, $F(a\mid\mathbf{U})$ a $|\mathcal{U}|\times|\mathcal{U}|$ diagonal matrix whose $s$th diagonal element is $f(a\mid u_{s})$, and $\mathbf{e}$ an all-one column vector of length $|\mathcal{U}|$. Without loss of generality, we assume that $\mathbf{W},\mathbf{Z},\mathbf{U}$ dimensions are equal. With these notations, Eq.~\ref{eq.uh} and~\ref{eq.uq} translate into the following linear equation system:
\begin{align}
	h_{0}^{\top}(\mathbf{W},a)\mathcal{P}(\mathbf{W}\mid \mathbf{U},a)=\mathbb{E} \left[ Y\mid \mathbf{U},a \right] &=\mathcal{P}(Y=1\mid \mathbf{U},a), \label{eq.uh_matrix}\\
	q_{0}^{\top}(\mathbf{Z},a)\mathcal{P}(\mathbf{Z}\mid \mathbf{U},a)F(a\mid \mathbf{U})&=\mathbf{e}^{\top} \label{eq.uq_matrix}
\end{align}
Then Eq.~\ref{eq.h} and~\ref{eq.q} translate into the following linear equation system:
\begin{align}
	h_{0}^{\top}(\mathbf{W},a)\mathcal{P} (\mathbf{W}\mid \mathbf{Z},a)=\mathbb{E} \left[ Y\mid \mathbf{Z},a\right] &=\mathcal{P} (Y=1\mid \mathbf{Z},a), \label{eq.h_matrix}\\
	q_{0}^{\top}(\mathbf{Z},a)\mathcal{P} (\mathbf{Z}\mid \mathbf{W},a)F(a\mid \mathbf{W})&=\mathbf{e}^{\top} \label{eq.q_matrix}
\end{align}
Since $\mathbf{W}\perp(\mathbf{Z},A)|\mathbf{U}$ and $\mathbf{Z}\perp Y|(\mathbf{U},A)$, we have
$$
\begin{aligned}
	\mathcal{P}(\mathbf{W}\mid \mathbf{Z},a)&=\mathcal{P}(\mathbf{W}\mid \mathbf{U})\mathcal{P}(\mathbf{U}\mid \mathbf{Z},a)\\
	\mathcal{P}(Y=1\mid \mathbf{Z},a)&=\mathcal{P}(Y=1\mid \mathbf{U},a)\mathcal{P}(\mathbf{U}\mid \mathbf{Z},a)\\
\end{aligned}
$$
Bring into the Eq.\ref{eq.h_matrix}, we have
\begin{equation}\label{eq.uh_matrix1}
    h_{0}^{\top}(\mathbf{W},a)\mathcal{P} (\mathbf{W}\mid \mathbf{U})\mathcal{P} (\mathbf{U}\mid \mathbf{Z},a)=\mathcal{P} (Y=1\mid \mathbf{U},a)\mathcal{P} (\mathbf{U}\mid \mathbf{Z},a)
\end{equation}

Therefore, if $\mathcal{P} (\mathbf{U}\mid \mathbf{Z},a)$ is singular matrix, then Assumption~\ref{assum:bridge} (1) does not hold. And we find solving the systems of linear equations~\ref{eq.uh_matrix} and~\ref{eq.uh_matrix1}, the solution space is different.

Besides, by $(\mathbf{Z},A)\perp \mathbf{W}|\mathbf{U}$, we have
$$
\begin{aligned}
	\mathcal{P} (\mathbf{Z}\mid \mathbf{W},a)&=\mathcal{P} (\mathbf{Z}\mid \mathbf{U},a)\mathcal{P} (\mathbf{U}\mid \mathbf{W})\\
	F^{-1}(a\mid \mathbf{W})&=F^{-1}(a\mid \mathbf{U})\mathcal{P} (\mathbf{U}\mid \mathbf{W})\\
\end{aligned}
$$
Bring into the Eq.\ref{eq.q_matrix}, as long as $\mathcal{P} (\mathbf{U}\mid \mathbf{W})$ is invertible matrix which implys Assumption~\ref{assum:bridge} (1) holds, we have
$$
\begin{aligned}
	\mathbf{e}^{\top}&=q_{0}^{\top}(\mathbf{Z},a)\mathcal{P} (\mathbf{Z}\mid \mathbf{W},a)F(a\mid \mathbf{W})\\
	&=q_{0}^{\top}(\mathbf{Z},a)\mathcal{P} (\mathbf{Z}\mid \mathbf{W},a)\mathcal{P} ^{-1}(\mathbf{U}\mid \mathbf{W})F(a\mid \mathbf{U})\\
	&=q_{0}^{\top}(\mathbf{Z},a)\mathcal{P} (\mathbf{Z}\mid \mathbf{U},a)F(a\mid \mathbf{U})\\
\end{aligned}
$$

% \begin{figure}[H]
%     \centering
%     \includegraphics[width=0.5\textwidth]{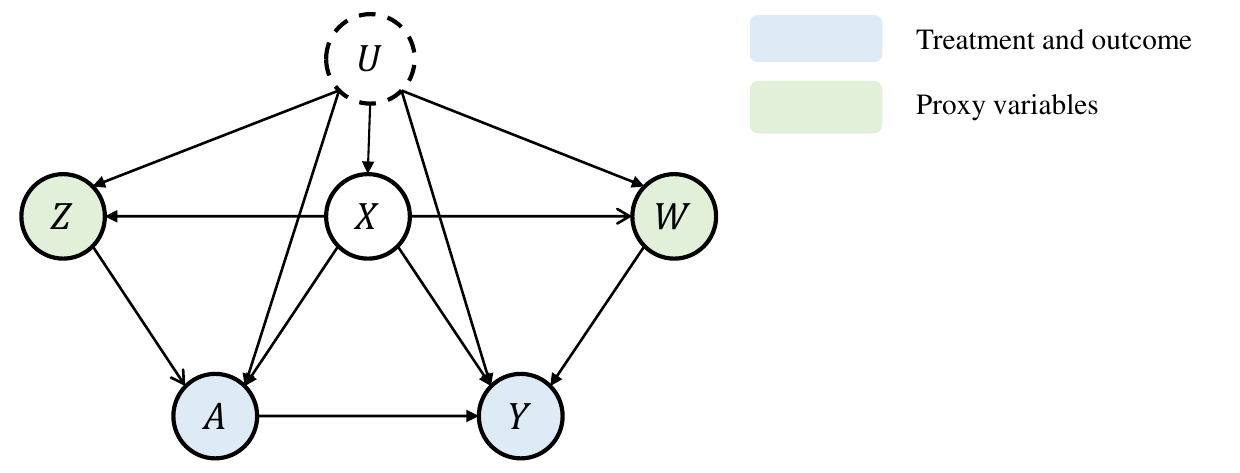}
%     \label{fig:DAG}
%     \caption{A typical causal diagram for proxy variables.}
% \end{figure}

\begin{example}
$$
\mathcal{P} \left( A \right) =\left( \begin{matrix}
	\frac{1}{2}&		\frac{1}{2}\\
\end{matrix} \right) \,\,  P\left( \mathbf{U}\mid \mathbf{Z},a \right) =\left( \begin{matrix}
	8-2i&		8-2i\\
	2+2i&		2+2i\\
\end{matrix} \right) /10 \,\, \mathcal{P} \left( \mathbf{Z}\mid A \right) =\left( \begin{matrix}
	\frac{2}{3}&		\frac{3}{7}\\
	\frac{1}{3}&		\frac{4}{7}\\
\end{matrix} \right) 
$$
$$
\mathcal{P} (Y=1,W\mid \mathbf{U},a_i)=\left( \begin{matrix}
	20-6i&		54-22i\\
	64-24i&		40-4i\\
\end{matrix} \right) /100,
$$
$$
\mathcal{P} (Y=0,W\mid \mathbf{U},a_i)=\left( \begin{matrix}
	6i&		22i-14\\
	24+16i&		2o+4i\\
\end{matrix} \right) /100
$$
\end{example}
\begin{proof}
Easy to obtain
$$
\begin{aligned}
	\mathcal{P} (W\mid \mathbf{U},a_i)&=\mathcal{P} (Y=1,W\mid \mathbf{U},a_i)+\mathcal{P} (Y=0,W\mid \mathbf{U},a_i)\\
	&=\left( \begin{matrix}
	\frac{1}{5}&		\frac{2}{5}\\
	\frac{4}{5}&		\frac{3}{5}\\
\end{matrix} \right) =\mathcal{P} (W\mid \mathbf{U}) 
\end{aligned}
$$
And 
$$
\mathcal{P} (Y=1\mid \mathbf{U},a_i)=\left( \begin{matrix}
	84-30i&		94-36i\\
\end{matrix} \right) /100
$$
Bring to Eq.~\ref{eq.uh_matrix}, we have
$$
h_{0}^{\top}(\mathbf{W},a_i)\left( \begin{matrix}
	\frac{1}{5}&		\frac{2}{5}\\
	\frac{4}{5}&		\frac{3}{5}\\
\end{matrix} \right) =\left( \begin{matrix}
	84-30i&		94-36i\\
\end{matrix} \right) /100
$$
Therefore,
$$
h_{0}^{\top}(\mathbf{W},a)=\left( \begin{matrix}
	1.24-0.54i&		0.74-0.24i\\
\end{matrix} \right) 
$$
Bring to Eq.~\ref{eq.uh_matrix1}, we have
$$
h_{0}^{\top}(\mathbf{W},a)\left( \begin{matrix}
	\frac{1}{5}&		\frac{2}{5}\\
	\frac{4}{5}&		\frac{3}{5}\\
\end{matrix} \right) \left( \begin{matrix}
	\frac{4}{5}&		\frac{4}{5}\\
	\frac{1}{5}&		\frac{1}{5}\\
\end{matrix} \right) =\frac{1}{100}\left( \begin{matrix}
	84-30i&		94-36i\\
\end{matrix} \right) \left( \begin{matrix}
	\frac{4}{5}&		\frac{4}{5}\\
	\frac{1}{5}&		\frac{1}{5}\\
\end{matrix} \right) 
$$
Obviously, the equation has infinite solutions.

Following the same derivation as before, by solving Eq.~\ref{eq.uq_matrix} or Eq.~\ref{eq.q_matrix}, we obtain $q$. Although the solution space of $q$ also has infinitely many solutions, the solution spaces of the two equations are the same.
\end{proof}
